# Supplementary material for: CLOSE: A Calibrated Label-free Online Self-Evaluating Verifier for Object Hallucination in Vision-Language Models
Source: arXiv:2611.28589 source file (2026-11-21)
Supplement: Supplementary file 1 [file appendix_setup.tex]

\makeatletter
\@addtoreset{table}{section}
\@addtoreset{figure}{section}
\@addtoreset{algorithm}{section}
\makeatother
\setcounter{table}{0}\setcounter{figure}{0}
\renewcommand{\thetable}{\thesection\arabic{table}}
\renewcommand{\thefigure}{\thesection\arabic{figure}}
\renewcommand{\thealgorithm}{\thesection\arabic{algorithm}}
\renewcommand{\topfraction}{0.9}\renewcommand{\bottomfraction}{0.8}\renewcommand{\textfraction}{0.07}
\renewcommand{\floatpagefraction}{0.75}\renewcommand{\dbltopfraction}{0.9}\renewcommand{\dblfloatpagefraction}{0.75}
\setcounter{topnumber}{4}\setcounter{totalnumber}{6}\setcounter{dbltopnumber}{3}
\raggedbottom
\makeatletter
\setlength{\@fptop}{0pt}\setlength{\@fpsep}{14pt plus 2pt}\setlength{\@fpbot}{0pt plus 1fil}
\setlength{\@dblfptop}{0pt}\setlength{\@dblfpsep}{14pt plus 2pt}\setlength{\@dblfpbot}{0pt plus 1fil}
\makeatother
